# Supplementary material for: Universal Wait-Free Memory Reclamation
Source: arXiv:2001.01999 source file (2020-01-12)
Supplement: Supplementary file 1 [file appendix.tex]

\section{Artifact appendix}

\subsection{Abstract}
The artifact includes our extended version of the benchmark~\cite{IBRPaper}.
It includes our new WFE scheme as well as existing schemes: HE, HP, EBR, and 
2GEIBR. The test set of lock-free data structures is extended with KP and
CRTurn wait-free queues.
The benchmark requires Linux with libjemalloc and libhwloc
(on an x86\_64 machine that supports cmpxchg16b). The gcc
compiler must support C++11 as well as extended inline assembly
features for cmpxchg16b (we tested gcc 8.3.0).

\subsection{Artifact check-list (meta-information)}

\begin{itemize}
\item \textbf{Algorithm:} New algorithm, Wait-Free Eras (WFE).
\item \textbf{Program:} The benchmark with WFE implementation.
\item \textbf{Compilation:} gcc with GCC\_ASM\_FLAG\_OUTPUT and C++11 support.
\item \textbf{Binary:} Linux ELF (x86\_64) executables.
\item \textbf{Run-time environment:} Ubuntu 18.04.3 LTS.
\item \textbf{Hardware:} Any multi-core x86\_64 with cmpxchg16b support; we tested it on 4x24 Intel Xeon~E7-8890~v4 (2.20GHz).
\item \textbf{Execution:} The execution time is passed through a program parameter.
\item \textbf{Output:} The output is produced in the CSV format. PDF plots
can be generated from CSV files.
\item \textbf{Experiments:} A single python script runs all presented test cases.
\item \textbf{Workflow frameworks used?:} No.
\item \textbf{Publicly available?:} Yes.
\item \textbf{Artifacts publicly available?:} Yes.
\item \textbf{Artifacts functional?:} Yes.
\item \textbf{Artifacts reusable?:} Yes.
\item \textbf{Results validated?:} Yes.
\end{itemize}

\subsection{Description}

\subsubsection{How delivered}
The artifact is available through the public repository:

\url{https://github.com/rusnikola/wfe}.

\subsubsection{Hardware dependencies}
Any multi-core x86\_64 with cmpxchg16b support; we tested the benchmark on 4x24 Intel Xeon~E7-8890~v4 (2.20GHz). For the Leak Memory experiment, 256GB of RAM is recommended, albeit RAM can still be much smaller if occasional outliers are acceptable.

\subsubsection{Software dependencies}
Linux with gcc (C++11 and GCC\_ASM\_FLAG\_OUTPUT support), python, libjemalloc, and libhwloc. In our setup with Ubuntu 18.04.3, the following packages were installed: g++-8, gcc-8, libhwloc-dev, libjemalloc-dev, python. (The default gcc version was set to 8.)
To draw charts, R is required: littler, r-cran-plyr, r-cran-ggplot2.

\subsection{Installation}
\begin{verbatim}
make [Release Version]
make debug [Debug Version]
\end{verbatim}

\subsection{Experiment workflow}

\begin{itemize}
\item Compile the benchmark.
\item Run tests. We provide testscript\_wfe.py which
runs all tests presented in the paper.
\item For individual tests,
you can also invoke tests directly. For example, for WFE's
hash map test (10 seconds):
\begin{verbatim}
./bin/main -i 10 -m 3 -v -r 1 -o hashmap.csv
           -t 4 -d tracker=WFE
\end{verbatim}

For HE's hash map:
\begin{verbatim}
./bin/main -i 10 -m 3 -v -r 1 -o hashmap.csv
           -t 4 -d tracker=HE
\end{verbatim}

(You can see all options by running ./bin/main -h.)

\item Plot the results. See below.

\end{itemize}

\subsection{Evaluation and expected result}

Throughput and the number of unreclaimed objects of WFE
should roughly correspond to HE. Other algorithms such as 2GEIBR and EBR
should have relatively similar performance to WFE and HE, i.e., the gap
is typically not very large.
HP, on the other hand, should typically have significantly worse
throughput but a smaller number of unreclaimed objects.

\textbf{Running all tests:}

\begin{verbatim}
cd ./ext/parharness/scripts
mkdir -p data/final
nohup ./testscript_wfe.py &
\end{verbatim}

The results will be in data/final/*.csv.
Note that this script takes long time to complete. For rough
results, the number of iterations in testscript\_wfe.py can be reduced.

\textbf{Drawing PDF plots:}

\begin{verbatim}
mv ./ext/parharness/scripts/data/final
       ./data/final
cd ./data/scripts
./genplots.sh
\end{verbatim}

PDF plots will be placed in ./data/final/*.pdf.
Note that genplots.sh runs *.R scripts from the same directory.
These scripts are adjusted for the parameters in
./testscript\_wfe.py.
When you change ./testscript\_wfe.py, these scripts may need to be changed
accordingly.

\subsection{Experiment customization}
The original benchmark we used~\cite{IBRPaper} is highly-customizable. New
reclamation schemes can be added to src/trackers (we added WFE), whereas
new data structure tests can be added to src/rideables (we added KP and CRTurn
queues).
